# Supplementary material for: Signal Reconstruction from Modulo Observations
Source: arXiv:1812.00557 source file (2019-07-17)
Supplement: Supplementary file 1 [file appendix.tex]

\section{Appendix}
\label{sec:append}
